# Supplementary material for: High flexoelectric constants in Janus transition-metal dichalcogenides
Source: arXiv:2208.09640 source file (2022-08-20)
Supplement: Supplementary file 1 [file Appendix.tex]

\section{Phase transition}
  \noindent The initial configuration of the system has $N\times N \times N$ unit cells. $N$ is the number of primitive cells in one direction of Cartesian coordinate system. The BaO-terminated primitive cell constructed in rhombohedral phase. The simulations are carried with a temperature and pressure constraints.  The relaxation time for thermostat and barostat are set as $0.1$ ps. The shells are assigned with a mass of 2 atomic units, which ensure the natural vibrational frequency of an-harmonic spring is well above the frequency of whole domain. This setting makes the shells to react with the electrostatic environment. The time step is set to 0.4 fs to record the atomic motions involving in high vibration frequency of an-harmonic spring. The interaction cut-off distance used is $16~\text{\AA}$. The accuracy of Ewald summation sets to $1\times10^{-6}$ for calculating long range Coulombic interaction in K-space. Periodic boundary conditions are imposed in all directions (unless otherwise stated) to remove surface effect to study the phase transition. The system is first equilibrated for 10000 steps at 80 K, followed by simulation run of 450000 steps. During the simulation run the system is heated from 80 K to 450 K with a constant rate. Atmospheric pressure of 1 bar imposed on the system. The lattice constant of the primitive cell is obtained by analyzing the simulation box size and shape during the heating period. Figure A.1 presents the temperature dependent lattice parameters of primitive cell extracted from the system with different sizes. Systems with 7$\times$7$\times$7, 10$\times$10$\times$10, 13$\times$13$\times$13 and 15$\times$15$\times$15 primitive cells have 3430, 10000, 21970 and 33750 atoms, respectively.\par  
\noindent Figure A.1 shows the variation of lattice parameter with temperature for different size samples. The increase in temperature changes the lattice parameter, which correspond to changes in the crystal structure. From the simulation results (Figure A.1a), the phase transition sequence Rhombohedral (R) $\rightarrow$ Orthorhombic (O) $\rightarrow$ Tetragonal (T) $\rightarrow$ Cubic (C) is correctly captured. The numerical value of lattice parameter has significant perturbations for system consist of $7\times7\times7$ cells. These perturbations are due to the unstable oscillations of atoms during the maintenance of thermal and pressure constraints. The variation of lattice parameter in Figure A.1b-A.1d represent that, the thermal and pressure induced perturbations are sufficiently relaxed with the increase in sample size. The transition temperature comparison is tabulated in Table A.1. The  prediction from core-shell model with parameters from Table.1 produce the transition temperatures in agreement with the experimental data for R $\rightarrow$ O and O $\rightarrow$ T phase change. A difference of $40$ K is found for the transition temperature from T $\rightarrow$ C with experiment.  Nevertheless, the predictions from present study have a better agreement with experiment values comparing to other MD studies. Figure A.3 suggests that system with total number of atoms larger than $10000$ is required to get a stable and correct estimation of phase change. The variation in lattice parameter alters the barycenter of all positive charges and barycenter of all negative charges. The non-zero  relative distance between the centers of positive and negative charges induce a non-zero dipole moment.  Furthermore, for ferroelectric material the electronic polarizability has significant contribution to the overall polarization. \par
\noindent Figure A.2 presents the three components of absolute averaged spontaneous polarization. Its expected that the spontaneous polarization has a size dependent behavior, as it derived from the atom coordinates. The calculated absolute spontaneous polarization for crystal phase R, O and T are 0.259, 0.23 and 0.195 $C/M^2$, respectively. These values fall within the range of experimental values, 0.13 to 0.19, 0.14 to 0.25 and 0.17 to 0.27 $C/M^2$\cite{kwei1993structures} \cite{shirane1952transition}, expect for the rhombohedral phase the core-shell model overestimates the value by 26 \%.  

\begin{center}
	\begin{figure}[h]
		\begin{center}
			\subfigure[7$\times$7$\times$7 cells]{\includegraphics[width=0.49 \linewidth]{Fig_A01_1.eps}}
			\subfigure[10$\times$10$\times$10 cells]{\includegraphics[width=0.49 \linewidth]{Fig_A01_2.eps}}
			\subfigure[13$\times$13$\times$13 cells]{\includegraphics[width=0.49 \linewidth]{Fig_A01_3.eps}}
			\subfigure[15$\times$15$\times$15 cells]{\includegraphics[width=0.49 \linewidth]{Fig_A01_4.eps}}
		\end{center}
		\caption{Temperature depended lattice parameters ({\AA}) of different size samples}
	\end{figure}
\end{center}

\begin{center}
	\begin{figure}[h]
		\begin{center}
			\subfigure[7$\times$7$\times$7 cells]{\includegraphics[width=0.49 \linewidth]{Fig_A02_1.eps}}
			\subfigure[10$\times$10$\times$10 cells]{\includegraphics[width=0.49 \linewidth]{Fig_A02_2.eps}}
			\subfigure[13$\times$13$\times$13 cells]{\includegraphics[width=0.49 \linewidth]{Fig_A02_3.eps}}
			\subfigure[15$\times$15$\times$15 cells]{\includegraphics[width=0.49 \linewidth]{Fig_A02_4.eps}}
		\end{center}
		\caption{Temperature depended absolute averaged spontaneous polarization ($C/m^2$) of different size samples}
	\end{figure}
\end{center}

\begin{figure}
	\centering
	\includegraphics[width=0.55\linewidth]{Fig_A03.eps}
	\caption{Illustration of size depended phase transition temperatures (K) of $\text{BaTiO}_3$} 
	%\label{Figure}
\end{figure}\par

\begin{center}
	\begin{table}
		\captionof{table}{$\text{BaTiO}_3$ transition temperature comparison (K)}
%		\begin{tabular}{c c c c c c}
%			\hline
%			\hline
%			Transition phase & This study  & This study  & \textcolor{blue}{Anisotropic}  & \textcolor{blue}{ReaxFF } & Experiment \cite{lemanov1996phase} \\
%			&(Table .1)&(parameters\cite{sepliarsky2005atomic})& (Tinte \cite{tinte1999atomistic}) & (Goddard \cite{goddard2002reaxff}) &  \\
%			R $\rightarrow$ O & 180 & 190 & 80 & \textcolor{blue}{197} & 183 \\
%			O $\rightarrow$ T & 267 & 225 & 120 & \textcolor{blue}{237} & 278\\
%			T $\rightarrow$ C & 353 & 346 & 180 & \textcolor{blue}{290} & 393\\
%			\hline
%			\hline
%		\end{tabular}
		\centering
		\begin{tabular}{l c c c}
			\hline
			\hline
			Study  & R $\rightarrow$ O & O $\rightarrow$ T & T $\rightarrow$ C \\
			This study (Table 1.) & 180 & 267 & 353 \\
			This study (parameters~\cite{sepliarsky2005atomic}) & 190 & 225 & 346 \\
			\textcolor{blue}{Anisotropic}(Tinte \cite{tinte1999atomistic}) & 80 & 120 & 180 \\
			\textcolor{blue}{ReaxFF }(Goddard \cite{goddard2002reaxff}) & \textcolor{blue}{197} & \textcolor{blue}{237} & \textcolor{blue}{290} \\
			Experiment \cite{lemanov1996phase} & 183 & 279 & 393 \\
			\hline
			\hline
		\end{tabular}
	\end{table}
\end{center}
